# Supplementary material for: NetBooster: Empowering Tiny Deep Learning By Standing on the Shoulders of Deep Giants
Source: arXiv:2306.13586 source file (2023-06-23)
Supplement: Supplementary file 1 [file 6-Supple.tex]

\section{NetBooster as a General Technique to Improve Network Performance}
\label{app:more model}
Existing works have shown that although larger networks normally suffer from over-fitting instead of under-fitting, increasing the network capacity can still lead to non-trivially performance improvement~\cite{liu2021swin,he2016deep,liu2021swin2}. To validate whether NetBooster has the potential as a general technique to boost neural networks' performance, we further validate the NetBooster on ResNet-50~\cite{he2016deep} and DeiT-Tiny~\cite{touvron2021training} on the ImageNet dataset with input resolution 224. 

\begin{table}[t]
    \centering
    % \vspace{-3em}
    \caption{Evaluating NetBooster's performance on ResNet-50 and DeiT-Tiny. }
    \resizebox{0.8\linewidth}{!}{
    \begin{tabular}{c|c|c}
    \toprule
      Network & Training method & Accuracy\\
      \midrule
      \multirow{2}{*}{ResNet-50} & Vanilla & 77.6 \\
      & NetBooster & \textbf{78.0} \\
      \midrule
      \multirow{2}{*}{DeiT-Tiny} & Vanilla & 72.2 \\ 
      & NetBooster & \textbf{73.7} \\
      \bottomrule
    \end{tabular}
    }
    \label{tab:resnet50}
    % \vspace{-2em}
\end{table}

\textbf{Experiments setting}: We follow the training setting in~\cite{he2016deep} and~\cite{touvron2021training} to train ResNet-50 and DeiT-Tiny, respectively. We follow the proposed setting to expand 50\% of blocks in ResNet-50 and DeiT-Tiny uniformly. Specifically, for ResNet-50, we expand the first layer into the inverted residual block with a depthwise convolution kernel size of 3, expansion ratio 6 in the first layer in the selected blocks. For DeiT-Tiny, we expand the first fully connected layer in the feedforward network of the selected blocks into two fully connected layers with an expansion ratio of 6. We set $E_d$ to 20\% of the total training epochs. 

\begin{figure}[!t]
    % \vspace{-2em}
    \centering
    \includegraphics[width=0.5\linewidth]{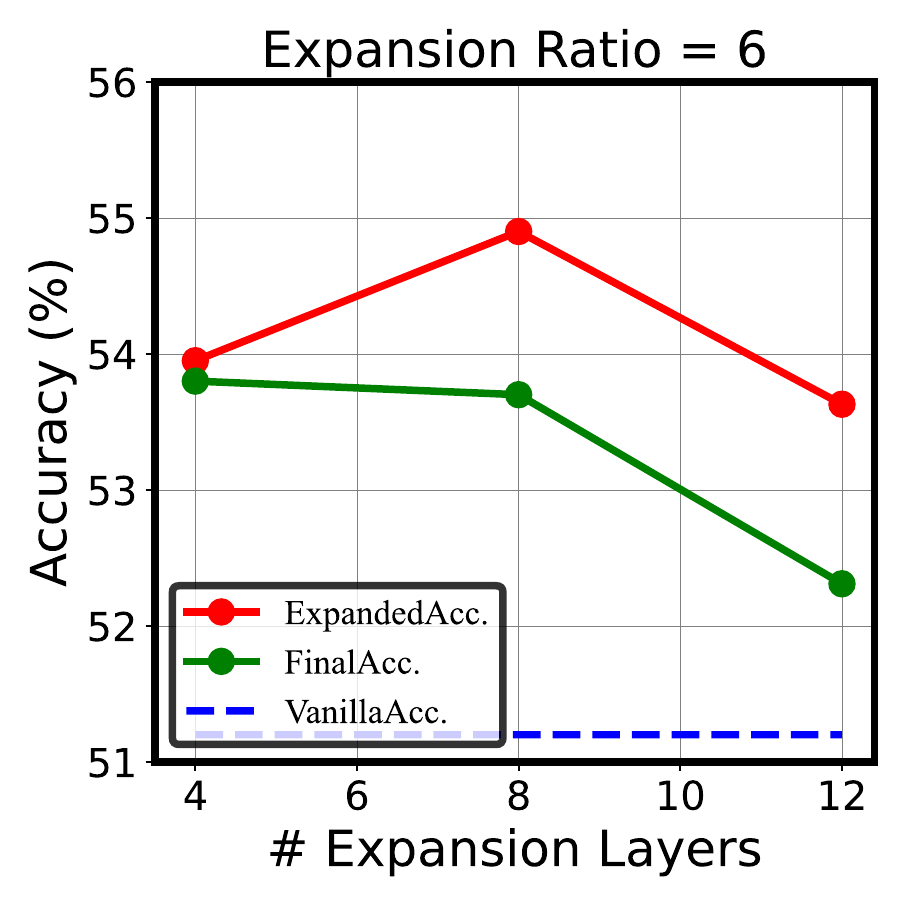}
    % \vspace{-1em}
    \caption{Visualization of the expanded accuracy (i.e., the accuracy of the expanded network) and final accuracy when using different numbers of expand blocks with an expansion ratio 6. }
    \label{fig:expansion-vis}
    % \vspace{-4em}
\end{figure}

\textbf{Results}: As shown in Table~\ref{tab:resnet50}, NetBooster leads to 0.4\% higher accuracy over vanilla training on the large-scale DNN (i.e., ResNet-50) and 1.5\% higher accuracy over the attention-based vision transformer (i.e., DeiT-Tiny), showing its promising potential in boosting all DNNs' performance.

\section{Number of Expansion Layers}
\label{app:number of layer}
The other factor that controls the deep giant's capacity is the number of expansion layers. We evaluate the relationship between the expansion ratio and the final performance on MobileNetV2-Tiny and the ImageNet dataset with an input resolution of 144. As shown in Fig.~\ref{fig:expansion-vis}, we observe that with various numbers of expansion layers, (1) networks boosted by the expansion-then-contraction strategy in NetBooster can constantly surpass the performance of vanilla networks, proving the NetBooster's effectiveness, (2) the expanded network performance (ExpandAcc.) increase first then decrease. We suspect the decrease in the expanded network accuracy is due to the overly deep network makes it challenging to train the network effectively, and (3) the boosted network performance (FinalAcc.) also has the increase-then-decrease pattern, validating our selected number of expansion layers.
